# Supplementary material for: D3G: Exploring Gaussian Prior for Temporal Sentence Grounding with Glance Annotation
Source: arXiv:2308.04197 source file (2023-08-08)
Supplement: Supplementary file 1 [file appendix.tex]

\documentclass[10pt,twocolumn,letterpaper]{article}

\usepackage{iccv}
\usepackage{times}
\usepackage{epsfig}
\usepackage{graphicx}
\usepackage{amsmath}
\usepackage{amssymb}
\usepackage{multirow}
\usepackage{booktabs}

% Include other packages here, before hyperref.

% If you comment hyperref and then uncomment it, you should delete
% egpaper.aux before re-running latex.  (Or just hit 'q' on the first latex
% run, let it finish, and you should be clear).
\usepackage[pagebackref=true,breaklinks=true,letterpaper=true,colorlinks,bookmarks=false]{hyperref}

\iccvfinalcopy % *** Uncomment this line for the final submission

 % *** Enter the ICCV Paper ID here

% Pages are numbered in submission mode, and unnumbered in camera-ready
\ificcvfinal\pagestyle{empty}\fi

\newcommand{\delete}[1]{{\color{red} }} %delete
% \newcommand{\blue}[1]{{\color{blue} #1}} %modify 
 %modify for final paper

\begin{document}
\input{D3G/Sections/6_supp}
\end{document}
